# Supplementary material for: Efficient Second-Order TreeCRF for Neural Dependency Parsing
Source: arXiv:2005.00975 source file (2020-06-29)
Supplement: Supplementary file 1 [file appendix.tex]

\section{Appendix (See Supplement Document)}
\label{section:appendix}
